# Supplementary material for: On the independence ratio of distance graphs
Source: arXiv:1401.7183 source file (2014-01-28)
Supplement: Supplementary file 1 [file table-appendix.tex]

\begin{longtable}[h]{@{\extracolsep{\fill}}r|c@{\ }c@{\ }c@{\ }c@{\ }c@{\ }c@{\ }c@{\ }c@{\ }c@{\ }c@{\ }c@{\ }c@{\ }c@{\ }c@{\ }c@{\ }c@{\ }c@{\ }c@{\ }c@{\ }c@{\ }c@{\ }c@{\ }c@{\ }c@{\ }c@{\ }c@{\ }c@{\ }c@{\ }c@{\ }c@{\ }c@{\ }c@{\ }c@{\ }c@{\ }c@{\ }c@{\ }c@{\ }c@{\ }c@{\ }c@{\ }}
 $k \setminus i$ & $1$& $2$& $3$& $4$& $5$& $6$& $7$& $8$& $9$& $10$& $11$& $12$& $13$& $14$& $15$& $16$& $17$& $18$& $19$& $20$& $21$& $22$& $23$& $24$& $25$& $26$& $27$& $28$& $29$& $30$& $31$& $32$& $33$& $34$& $35$& $36$& $37$& $38$& $39$& $40$\\\hline
$1$ & { 1/ 4} & { 1/ 3} & { 1/ 3} & { 2/ 7} & { 1/ 3} & { 1/ 3} & { 3/10} & { 1/ 3} & { 1/ 3} & { 4/13} & { 1/ 3} & { 1/ 3} & { 5/16} & { 1/ 3} & { 1/ 3} & { 6/19} & { 1/ 3} & { 1/ 3} & { 7/22} & { 1/ 3} & { 1/ 3} & { 8/25} & { 1/ 3} & { 1/ 3} & { 9/28} & { 1/ 3} & { 1/ 3} & {10/31} & { 1/ 3} & { 1/ 3} & {11/34} & { 1/ 3} & { 1/ 3} & {12/37} & { 1/ 3} & { 1/ 3} & {13/40} & { 1/ 3} & { 1/ 3} & {14/43} \\\hline
$2$ & { 2/ 7} && { 1/ 3} && { 4/11} && { 5/13} && { 2/ 5} && { 7/17} && { 8/19} && { 3/ 7} && {10/23} && {11/25} && { 4/ 9} && {13/29} && {14/31} && { 5/11} && {16/35} && {17/37} && { 6/13} && {19/41} && {20/43} && { 7/15} &\\\hline
$3$ & { 1/ 3} & { 2/ 5} & { 3/ 8} & { 1/ 3} & { 2/ 5} & { 4/11} & { 2/ 5} & { 5/13} & { 5/14} & { 2/ 5} & { 3/ 8} & { 2/ 5} & { 7/18} & { 7/19} & { 2/ 5} & { 8/21} & { 2/ 5} & { 9/23} & { 3/ 8} & { 2/ 5} & { 5/13} & { 2/ 5} & {11/28} & {11/29} & { 2/ 5} & {12/31} & { 2/ 5} & {13/33} & {13/34} & { 2/ 5} & { 7/18} & { 2/ 5} & {15/38} & { 5/13} & { 2/ 5} & {16/41} & { 2/ 5} & {17/43} & {17/44} & { 2/ 5} \\\hline
$4$ & { 2/ 7} && { 1/ 3} && { 1/ 3} && { 6/17} && { 7/19} && { 8/21} && { 9/23} && { 2/ 5} && {11/27} && {12/29} && {13/31} && {14/33} && { 3/ 7} && {16/37} && {17/39} && {18/41} && {19/43} && { 4/ 9} && {21/47} && {22/49} &\\\hline
$5$ & { 4/13} & { 3/ 7} & { 2/ 5} & { 3/ 8} & { 5/12} & { 1/ 3} & { 3/ 7} & { 2/ 5} & { 3/ 7} & { 7/17} & { 9/23} & { 8/19} & { 2/ 5} & { 3/ 7} & { 9/22} & { 3/ 7} & { 5/12} & { 2/ 5} & {11/26} & {11/27} & { 3/ 7} & {12/29} & { 3/ 7} & {13/31} & {13/32} & {14/33} & { 7/17} & { 3/ 7} & { 5/12} & { 3/ 7} & { 8/19} & {16/39} & {17/40} & {17/41} & { 3/ 7} & {18/43} & { 3/ 7} & {19/45} & {\color{red} 19/46} & {20/47} \\\hline
$6$ & { 1/ 3} && { 4/11} && { 3/ 8} && { 1/ 3} && { 6/17} && { 7/19} && { 3/ 8} && {11/29} && {12/31} && {13/33} && { 2/ 5} && {15/37} && {16/39} && {17/41} && {18/43} && {19/45} && {20/47} && { 3/ 7} && {22/51} && {23/53} &\\\hline
$7$ & { 3/10} & { 4/ 9} & { 7/19} & { 2/ 5} & { 3/ 7} & { 4/11} & { 7/16} & { 1/ 3} & { 4/ 9} & { 5/13} & { 4/ 9} & { 3/ 7} & {12/29} & {10/23} & {12/31} & {11/25} & {13/33} & { 4/ 9} & { 3/ 7} & { 4/ 9} & {13/30} & { 8/19} & { 7/16} & { 2/ 5} & {15/34} & { 3/ 7} & { 4/ 9} & {16/37} & { 4/ 9} & {17/39} & {20/47} & {18/41} & { 3/ 7} & {19/43} & {19/44} & { 4/ 9} & {10/23} & { 4/ 9} & { 7/16} & { 3/ 7} \\\hline
$8$ & { 6/19} && { 5/13} && { 2/ 5} && { 2/ 5} && { 1/ 3} && { 8/21} && { 9/23} && { 2/ 5} && { 2/ 5} && {11/29} && {12/31} && {13/33} && { 2/ 5} && { 2/ 5} && {19/47} && {20/49} && { 7/17} && {22/53} && {23/55} && { 8/19} &\\\hline
$9$ & { 1/ 3} & { 5/11} & { 5/14} & { 5/12} & { 2/ 5} & { 5/13} & { 4/ 9} & { 4/11} & { 9/20} & { 1/ 3} & { 5/11} & { 3/ 8} & { 5/11} & { 7/17} & { 3/ 7} & { 4/ 9} & {15/37} & {13/29} & { 5/13} & {14/31} & {16/41} & { 5/11} & {18/43} & { 5/11} & { 4/ 9} & {10/23} & {17/38} & { 5/12} & { 9/20} & { 2/ 5} & {19/42} & {11/26} & { 5/11} & { 4/ 9} & { 5/11} & {21/47} & {25/57} & {22/49} & {25/59} & {23/51} \\\hline
$10$ & { 4/13} && { 2/ 5} && { 7/17} && { 5/12} && {12/31} && { 1/ 3} && { 2/ 5} && {11/27} && {12/29} && { 5/12} && {17/43} && { 2/ 5} && {15/37} && {16/39} && {17/41} && { 5/12} && { 2/ 5} && {\color{red} 19/47} && {\color{red} 20/49} && {\color{red}  7/17} &\\\hline
$11$ & { 8/25} & { 6/13} & { 3/ 8} & { 3/ 7} & { 5/13} & { 2/ 5} & {13/31} & { 8/21} & { 5/11} & { 5/13} & {11/24} & { 1/ 3} & { 6/13} & {10/27} & { 6/13} & { 2/ 5} & {18/41} & { 3/ 7} & {18/43} & { 5/11} & { 2/ 5} & {16/35} & { 5/13} & {17/37} & {19/49} & { 6/13} & { 7/17} & { 6/13} & {23/53} & { 4/ 9} & { 5/11} & { 3/ 7} & {21/46} & {12/29} & {11/24} & { 2/ 5} & {23/50} & {13/31} & { 6/13} & { 7/16} \\\hline
$12$ & { 1/ 3} && {11/29} && { 8/19} && { 3/ 7} && { 3/ 7} && {14/37} && { 1/ 3} && {16/41} && {13/31} && {14/33} && { 3/ 7} && { 3/ 7} && {20/51} && {21/53} && {18/43} && {19/45} && {20/47} && { 3/ 7} && { 3/ 7} && { 2/ 5} &\\\hline
$13$ & { 5/16} & { 7/15} & { 7/18} & { 7/16} & { 2/ 5} & { 7/17} & { 2/ 5} & { 9/23} & {16/37} & { 2/ 5} & { 6/13} & { 2/ 5} & {13/28} & { 1/ 3} & { 7/15} & {12/31} & { 7/15} & {13/33} & {21/47} & { 5/12} & { 3/ 7} & {11/25} & { 7/17} & { 6/13} & { 2/ 5} & {19/41} & { 2/ 5} & {20/43} & {\color{red} 17/44} & { 7/15} & {24/59} & { 7/15} & {26/61} & {14/31} & { 4/ 9} & { 7/16} & { 6/13} & {14/33} & {25/54} & { 7/17} \\\hline
$14$ & {10/31} && { 7/19} && { 3/ 7} && {10/23} && { 7/16} && {17/41} && { 3/ 8} && { 1/ 3} && {18/47} && { 3/ 7} && {16/37} && {17/39} && { 7/16} && { 8/19} && {23/59} && {24/61} && { 3/ 7} && {22/51} && {23/53} && {24/55} &\\\hline
$15$ & { 1/ 3} & { 8/17} & { 2/ 5} & { 4/ 9} & { 9/22} & { 8/19} & { 7/17} & { 2/ 5} & {17/41} & {11/27} & {19/43} & { 7/17} & { 7/15} & { 9/23} & {15/32} & { 1/ 3} & { 8/17} & { 2/ 5} & { 8/17} & {15/37} & {24/53} & {\color{red} 16/39} & {24/55} & { 3/ 7} & { 8/19} & {13/29} & { 9/22} & { 7/15} & { 7/17} & {22/47} & {25/63} & {23/49} & { 2/ 5} & { 8/17} & {\color{red} 21/52} & { 8/17} & {29/69} & {16/35} & {31/71} & { 4/ 9} \\\hline
$16$ & { 6/19} && { 8/21} && {16/39} && {11/25} && { 4/ 9} && { 4/ 9} && {19/47} && { 7/18} && { 1/ 3} && {\color{red} 14/37} && {23/55} && {18/41} && {19/43} && { 4/ 9} && { 4/ 9} && {27/65} && {\color{red}  7/18} && { 9/23} && {30/71} && {25/57} &\\\hline
$17$ & {12/37} & { 9/19} & { 5/13} & { 9/20} & { 5/12} & { 3/ 7} & { 8/19} & { 9/22} & { 2/ 5} & {12/29} & {20/47} & {13/31} & {22/49} & { 8/19} & { 8/17} & { 5/13} & {17/36} & { 1/ 3} & { 9/19} & {11/28} & { 9/19} & {17/41} & {27/59} & {18/43} & {27/61} & { 8/19} & { 3/ 7} & { 7/16} & {\color{red}  5/12} & { 5/11} & {21/50} & { 8/17} & { 8/19} & {25/53} & {28/71} & {26/55} & {29/73} & { 9/19} & {12/29} & { 9/19} \\\hline
$18$ & { 1/ 3} && { 9/23} && { 2/ 5} && { 4/ 9} && {13/29} && { 9/20} && {22/51} && { 2/ 5} && { 2/ 5} && { 1/ 3} && {16/41} && {25/61} && { 4/ 9} && {21/47} && {22/49} && { 9/20} && {31/71} && {30/73} && { 2/ 5} && {\color{red} 23/59} &\\\hline
$19$ & {\color{red}  7/22} & {10/21} & { 3/ 8} & { 5/11} & {11/26} & {10/23} & { 3/ 7} & { 5/12} & { 3/ 7} & { 2/ 5} & { 7/17} & {14/33} & {23/53} & { 3/ 7} & { 5/11} & { 3/ 7} & { 9/19} & { 8/21} & {19/40} & { 1/ 3} & {10/21} & {12/31} & {10/21} & {19/45} & { 6/13} & {20/47} & {30/67} & { 3/ 7} & {10/23} & { 3/ 7} & {\color{red} 11/26} & { 4/ 9} & {23/54} & {17/37} & { 3/ 7} & { 9/19} & { 3/ 7} & {28/59} & {31/79} & {29/61} \\\hline
$20$ & {14/43} && { 2/ 5} && {11/27} && { 3/ 7} && {14/31} && { 5/11} && { 5/11} && { 8/19} && { 9/22} && {24/61} && { 1/ 3} && { 2/ 5} && {\color{red} 19/47} && {10/23} && {23/51} && {24/53} && { 5/11} && { 5/11} && {34/79} && { 9/22} &\\\hline
$21$ & { 1/ 3} & {11/23} & { 5/13} & {11/24} & { 3/ 7} & {11/25} & {13/30} & {11/26} & {10/23} & {11/27} & { 2/ 5} & { 3/ 7} & { 8/19} & {16/37} & {26/59} & {10/23} & {28/61} & {13/31} & {10/21} & { 9/23} & {21/44} & { 1/ 3} & {11/23} & {\color{red} 18/47} & {11/23} & { 3/ 7} & {33/71} & {22/51} & {33/73} & {23/53} & {11/25} & {10/23} & { 3/ 7} & {17/39} & {25/58} & { 9/20} & {13/30} & {19/41} & {10/23} & {10/21} \\\hline
$22$ & {\color{red}  8/25} && {19/49} && {12/29} && { 5/12} && { 5/11} && {16/35} && {11/24} && {27/61} && {\color{red} 17/41} && { 5/12} && {26/67} && { 1/ 3} && {28/71} && { 7/17} && {32/75} && { 5/11} && {26/57} && {27/59} && {11/24} && {38/85} &\\\hline
$23$ & {16/49} & {12/25} & {11/28} & { 6/13} & {22/53} & { 4/ 9} & { 7/16} & { 3/ 7} & {11/25} & {12/29} & {25/59} & { 2/ 5} & {25/61} & {17/39} & { 3/ 7} & {18/41} & {29/65} & {11/25} & {31/67} & { 7/17} & {11/23} & { 2/ 5} & {23/48} & { 1/ 3} & {12/25} & {20/51} & {12/25} & { 8/19} & {36/77} & {24/55} & {36/79} & {25/57} & { 4/ 9} & {11/25} & {36/83} & { 3/ 7} & {27/62} & {19/43} & { 7/16} & { 5/11} \\\hline
$24$ & { 1/ 3} && {\color{red} 11/29} && {13/31} && {11/26} && {26/59} && {17/37} && { 6/13} && { 6/13} && {29/67} && {19/45} && {11/26} && {\color{red}  5/13} && { 1/ 3} && {30/77} && {23/55} && {\color{red}  8/19} && {37/83} && {28/61} && {29/63} && { 6/13} &\\\hline
$25$ & {\color{red}  9/28} & {13/27} & { 2/ 5} & {13/28} & {13/32} & {13/29} & {15/34} & {13/30} & { 4/ 9} & {13/31} & { 4/ 9} & {\color{red} 11/27} & { 2/ 5} & {14/33} & {28/67} & {19/43} & {10/23} & { 4/ 9} & {32/71} & { 4/ 9} & {34/73} & {\color{red} 11/27} & {12/25} & {15/38} & {25/52} & { 1/ 3} & {13/27} & { 2/ 5} & {13/27} & {17/41} & {39/83} & {26/59} & {39/85} & {27/61} & {13/29} & { 4/ 9} & {39/89} & { 4/ 9} & { 3/ 7} & {10/23} \\\hline
$26$ & {18/55} && {12/31} && {14/33} && { 3/ 7} && { 3/ 7} && { 6/13} && {19/41} && {13/28} && {32/71} && {\color{red} 20/47} && { 3/ 7} && { 3/ 7} && {11/28} && {\color{red} 22/67} && {\color{red} 22/57} && {25/59} && {26/61} && {39/89} && { 6/13} && {31/67} &\\\hline
$27$ & { 1/ 3} & {14/29} & {23/59} & { 7/15} & { 7/17} & {14/31} & { 4/ 9} & { 7/16} & {17/38} & {14/33} & {13/29} & {12/29} & {29/69} & { 2/ 5} & {\color{red}  9/22} & { 4/ 9} & {31/73} & {21/47} & {11/25} & {13/29} & { 5/11} & {17/39} & {37/79} & {12/29} & {13/27} & {16/41} & {27/56} & { 1/ 3} & {14/29} & {17/43} & {14/29} & {\color{red} 25/61} & {42/89} & { 4/ 9} & { 6/13} & {29/65} & {14/31} & {30/67} & {42/95} & {13/29} \\\hline
$28$ & {\color{red} 10/31} && {13/33} && { 3/ 7} && {16/37} && {13/30} && {31/69} && {20/43} && { 7/15} && { 7/15} && {34/77} && {22/51} && {13/30} && {35/83} && { 2/ 5} && { 1/ 3} && {24/61} && { 3/ 7} && {28/65} && {\color{red} 29/67} && {44/97} &\\\hline
$29$ & {20/61} & {15/31} & {\color{red} 13/34} & {15/32} & { 5/12} & { 5/11} & {29/67} & {15/34} & { 9/20} & { 3/ 7} & {14/31} & {\color{red} 18/43} & {32/73} & {13/31} & { 2/ 5} & { 8/19} & {\color{red}  5/12} & {22/49} & {34/79} & {23/51} & { 4/ 9} & {14/31} & {38/83} & { 3/ 7} & { 8/17} & {13/31} & {14/29} & {\color{red} 12/31} & {29/60} & {\color{red}  1/99} & {15/31} & { 9/23} & {15/31} & {27/65} & { 9/19} & { 7/16} & {45/97} & {31/69} & { 5/11} & {32/71} \\\hline
$30$ & { 1/ 3} && { 2/ 5} && {28/67} && {17/39} && { 7/16} && {32/73} && { 7/15} && {22/47} && {15/32} && {37/81} && {\color{red} 23/53} && {24/55} && { 7/16} && {37/89} && {36/91} && {\color{red}  1/99} && { 2/ 5} && {41/97} && {10/23} && {\color{red} 31/71} &\\\hline
$31$ & {\color{red} 11/34} & {16/33} & { 7/18} & { 8/17} & { 8/19} & {16/35} & {\color{red} 14/33} & { 4/ 9} & {19/42} & {16/37} & { 5/11} & {\color{red} 19/45} & { 5/11} & {14/33} & {33/79} & { 2/ 5} & {\color{red} 21/50} & {18/41} & {\color{red} 11/26} & {24/53} & {37/85} & { 5/11} & {13/29} & { 5/11} & {41/89} & {\color{red} 25/59} & {43/91} & {14/33} & {15/31} & {13/33} & {31/64} & {\color{red}  1/99} & {16/33} & {\color{red} 26/67} & {16/33} & {29/69} & {29/61} & {22/51} & {41/88} & {33/73} \\\hline
$32$ & {22/67} && { 9/23} && {\color{red} 16/39} && {18/41} && {15/34} && { 3/ 7} && {36/79} && {23/49} && { 8/17} && { 8/17} && {13/29} && {25/57} && {26/59} && {15/34} && {\color{red}  7/17} && {38/97} && {\color{red}  1/99} && {\color{red}  9/23} && {38/91} && {32/73} &\\\hline
$33$ & { 1/ 3} & {17/35} & {15/38} & {17/36} & {17/40} & {17/37} & { 3/ 7} & {17/38} & { 5/11} & {17/39} & {21/46} & {\color{red} 20/47} & {16/35} & { 3/ 7} & {36/83} & { 3/ 7} & { 2/ 5} & {18/43} & {\color{red} 23/54} & { 5/11} & { 3/ 7} & {26/57} & {40/91} & {16/35} & {14/31} & {21/47} & {44/95} & { 3/ 7} & {46/97} & { 3/ 7} & {16/33} & { 2/ 5} & {33/68} & {\color{red}  1/99} & {17/35} & {\color{red} 28/71} & {17/35} & {31/73} & {41/86} & {\color{red} 32/75} \\\hline
$34$ & {\color{red} 12/37} && {\color{red}  5/13} && {17/41} && {19/43} && { 4/ 9} && { 4/ 9} && {37/83} && { 8/17} && {25/53} && {17/36} && { 6/13} && {41/93} && {27/61} && { 4/ 9} && { 4/ 9} && { 5/12} && {\color{red}  7/18} && {\color{red}  1/99} && {\color{red}  7/18} && {\color{red} 31/75} &\\\hline
$35$ & {24/73} & {18/37} & { 2/ 5} & { 9/19} & { 3/ 7} & { 6/13} & {19/44} & { 9/20} & { 4/ 9} & {18/41} & {11/24} & { 3/ 7} & {17/37} & {22/51} & {13/29} & {16/37} & {37/89} & { 2/ 5} & { 3/ 7} & {10/23} & {\color{red} 25/58} & {27/59} & {\color{red} 16/37} & {28/61} & {43/97} & {17/37} & { 5/11} & {11/25} & {27/58} & {16/37} & {39/82} & {\color{red} 40/97} & {17/35} & {\color{red} 22/57} & {35/72} & {\color{red}  1/99} & {18/37} & { 2/ 5} & {18/37} & { 3/ 7} \\\hline
$36$ & { 1/ 3} && {16/41} && {18/43} && { 4/ 9} && {21/47} && {17/38} && {38/87} && {41/89} && {26/55} && { 9/19} && { 9/19} && {44/97} && { 4/ 9} && {29/65} && {17/38} && {39/89} && { 8/19} && {15/38} && {\color{red}  1/99} && {\color{red} 30/77} &\\\hline
$37$ & {\color{red} 13/40} & {19/39} & {31/79} & {19/40} & {34/81} & {19/41} & {10/23} & {19/42} & {\color{red} 17/39} & {19/43} & {23/50} & {19/44} & { 6/13} & {23/53} & { 6/13} & {17/39} & {40/93} & {20/47} & { 2/ 5} & { 5/12} & {13/30} & {22/49} & {\color{red} 27/62} & {29/63} & {\color{red} 17/39} & { 6/13} & {25/56} & { 6/13} & {16/35} & {\color{red} 10/23} & {43/92} & {17/39} & {31/65} & {\color{red} 16/39} & {18/37} & {\color{red}  5/13} & {37/76} & {\color{red}  1/99} & {19/39} & {\color{red}  1/99} \\\hline
$38$ & {26/79} && {17/43} && {19/45} && {37/85} && {22/49} && { 9/20} && { 3/ 7} && {14/31} && { 9/19} && {28/59} && {19/40} && {27/58} && {25/56} && {30/67} && {31/69} && { 9/20} && {\color{red}  3/ 7} && {17/40} && {\color{red} 25/77} && {\color{red}  1/99} &\\\hline
$39$ & { 1/ 3} & {20/41} & {\color{red} 17/44} & {10/21} & {\color{red} 19/46} & {20/43} & { 7/16} & { 5/11} & {18/41} & { 4/ 9} & { 6/13} & {10/23} & {25/54} & {24/55} & {19/41} & {25/57} & {43/97} & {18/41} & {\color{red} 17/41} & { 2/ 5} & {23/54} & {22/51} & { 7/16} & { 6/13} & {18/41} & {31/67} & {29/66} & {19/41} & {40/89} & { 5/11} & {17/37} & {32/73} & {38/81} & {18/41} & {11/23} & {\color{red} 17/41} & {19/39} & {\color{red}  1/99} & {39/80} & {\color{red}  1/99} \\\hline
$40$ & {\color{red} 14/43} && { 2/ 5} && {20/47} && { 3/ 7} && {23/51} && {19/42} && {42/95} && {43/97} && {46/99} && {29/61} && {10/21} && {10/21} && {38/83} && {37/84} && {32/71} && {33/73} && {19/42} && { 3/ 7} && { 3/ 7} && {\color{red}  1/99} &\\\hline
$41$ & {28/85} & {21/43} & { 9/23} & {21/44} & { 5/12} & { 7/15} & {11/25} & {21/46} & {19/43} & {21/47} & {43/95} & { 7/16} & {13/28} & { 3/ 7} & {20/43} & {26/59} & {41/90} & {19/43} & {41/96} & {11/26} & { 2/ 5} & {\color{red} 27/65} & {29/66} & { 4/ 9} & {15/34} & {32/69} & {19/43} & {33/71} & {27/61} & {20/43} & {33/73} & {\color{red} 11/25} & { 6/13} & {34/77} & {\color{red} 37/80} & {19/43} & {35/73} & {18/43} & {20/41} & {\color{red}  1/99} \\\hline
$42$ & { 1/ 3} && {35/89} && { 3/ 7} && {22/51} && {24/53} && { 5/11} && { 5/11} && {27/62} && {26/57} && {10/21} && {31/65} && {21/44} && {37/79} && {37/82} && {43/97} && {34/75} && { 5/11} && { 5/11} && {19/44} && {\color{red} 27/65} &\\\hline
$43$ & {\color{red} 15/46} & {22/45} & {19/48} & {11/23} & {21/50} & {22/47} & {23/52} & {11/24} & { 4/ 9} & {22/49} & { 4/ 9} & {11/25} & {27/58} & {22/51} & { 7/15} & {27/61} & { 7/15} & { 4/ 9} & {29/66} & { 4/ 9} & {19/45} & { 2/ 5} & {36/85} & { 3/ 7} & {31/70} & {26/57} & { 4/ 9} & {34/73} & { 4/ 9} & { 7/15} & {41/92} & { 7/15} & {\color{red}  9/20} & {\color{red} 35/79} & {19/41} & { 4/ 9} & {\color{red} 13/28} & { 4/ 9} & {\color{red} 10/21} & {19/45} \\\hline
$44$ & {30/91} && {\color{red} 19/49} && { 8/19} && {23/53} && { 5/11} && {26/57} && {21/46} && { 3/ 7} && {35/78} && {29/62} && {32/67} && {11/23} && {11/23} && {\color{red} 43/94} && {\color{red}  7/16} && { 5/11} && {36/79} && {21/46} && {\color{red} 10/23} && {10/23} &\\\hline
$45$ & { 1/ 3} & {23/47} & { 2/ 5} & {23/48} & {11/26} & {23/49} & { 4/ 9} & {23/50} & {25/56} & {23/51} & {21/47} & {23/52} & { 7/15} & {23/53} & {29/62} & { 4/ 9} & {22/47} & {29/65} & {41/91} & {21/47} & {\color{red} 20/47} & { 8/19} & { 2/ 5} & {\color{red} 30/71} & { 4/ 9} & {26/59} & {33/74} & { 7/15} & {21/47} & {36/77} & {18/41} & {22/47} & {43/96} & {\color{red} 21/47} & {\color{red} 19/42} & {37/83} & {20/43} & {21/47} & {\color{red} 41/88} & {\color{red} 28/65} \\\hline
$46$ & {\color{red} 16/49} && {20/51} && {\color{red} 22/53} && {24/55} && {25/56} && {27/59} && {11/24} && {37/84} && {34/77} && {29/63} && {11/23} && {34/71} && {23/48} && {41/87} && {\color{red} 22/49} && {11/25} && {37/81} && {38/83} && {11/24} && {\color{red} 37/84} &\\\hline
$47$ & {\color{red}  8/25} & {24/49} & {13/33} & {12/25} & {23/54} & { 8/17} & {38/87} & { 6/13} & {13/29} & {24/53} & {22/49} & { 4/ 9} & {39/85} & {24/55} & {15/32} & { 3/ 7} & {23/49} & {30/67} & {41/89} & {22/49} & {17/39} & {26/59} & { 3/ 7} & {\color{red}  1/99} & {\color{red} 23/56} & {\color{red} 32/75} & {17/38} & {\color{red} 34/77} & {35/78} & {37/79} & {22/49} & {38/81} & {19/43} & {23/49} & {\color{red} 39/88} & {\color{red} 38/85} & {\color{red}  5/11} & {13/29} & { 7/15} & {22/49} \\\hline
$48$ & { 1/ 3} && {21/53} && {23/55} && {25/57} && {\color{red} 11/25} && {28/61} && {23/50} && {37/82} && {10/23} && {29/64} && { 8/17} && {35/73} && {12/25} && {12/25} && {\color{red} 41/89} && {\color{red} 23/52} && {\color{red} 29/66} && {39/85} && {40/87} && {23/50} &\\\hline
$49$ & {\color{red} 17/52} & {25/51} & {\color{red}  7/18} & {25/52} & { 3/ 7} & {25/53} & {\color{red} 25/58} & {25/54} & { 9/20} & { 5/11} & {23/51} & {25/56} & {37/82} & {25/57} & {31/66} & {\color{red} 22/51} & { 8/17} & {31/69} & { 8/17} & {32/71} & {29/65} & {23/51} & {\color{red} 22/51} & {13/31} & {\color{red}  1/99} & { 3/ 7} & {41/93} & { 7/16} & { 9/20} & {\color{red} 37/81} & {23/51} & {39/83} & {43/97} & { 8/17} & { 4/ 9} & { 8/17} & {\color{red} 41/92} & {\color{red} 40/89} & {\color{red} 21/46} & {41/91} \\\hline
$50$ & {\color{red} 17/53} && { 2/ 5} && { 8/19} && {26/59} && {23/52} && {29/63} && { 6/13} && { 6/13} && {\color{red} 30/71} && {29/65} && {\color{red} 45/98} && {12/25} && {37/77} && {25/52} && {\color{red} 43/93} && {\color{red} 24/53} && { 4/ 9} && {\color{red} 13/29} && {41/89} && { 6/13} &\\\hline
\end{longtable}
